# Supplementary material for: Generative Layout Modeling using Constraint Graphs
Source: arXiv:2011.13417 source file (2020-11-26)
Supplement: Supplementary file 1 [file appendix.tex]

\section{Layout Representation Details}
\label{app:layout_rep}

\paul{TODO: make a pass}

We use the \rplan and \lifull datasets to train and validate our method. These datasets contain a top-down orthographic view of the floors, also known as the plan-view. The first step is to find a simplified representation of these plans over which we learn the generative model.

\wamiq{Describe simplifying strategies}.

We further process this simplified plan to extract non-overlapping, adjacent quads\footnote{See Supplementary for details of our parsing process}. In this representation, as single room may be broken down into multiple rooms to satisfy the non-overlapping criterion. Thus, while parsing the floorplan, we also keep track of which boxes belong to the same-room, so that we can merge boxes that belong to the same room. 

From this representation, we can easily parse constraints between boxes - we already mentioned a constraint is whether two boxes are part of the same room, which is the same as the absence of a \wall. We can also have a \door constraint which means a door exists between two boxes, and hence the rooms containing those boxes. Important from an optimization perspective are the adjacency constraints - which boxes share a boundary. We decompose adjacency constraints into two disjoint sets: 1. Horizontal and 2. Vertical. A Horizontal(Vertical) constraint is imposed on two boxes if one box is to the left of (below) another box they share a vertical(horizontal) boundary. 

Each individual box can be thus be described completely by a five-tuple $\boxx = (\idxed{c}{i}, \idxed{x}{i}, \idxed{y}{i}, \idxed{w}{i}, \idxed{h}{i})$. We then quantize the tuple to a fixed-number of levels $L = 2^b$, where $b$ is the number of bits used to encode each element of the tuple. We use $b=6$ for a total of 64 levels. This allows use to treat each of the attributes as a discrete \textit{token} \cite{nash2020polygen, DBLP:conf/nips/RazaviOV19}. A floorplan is then a set of all these non-overlapping, quantized boxes. 

The constraints that occur between pairs of rooms/boxes can be represented by graphs with an edge occurring between a pair of boxes if they are constrained by adjacency, \door or \wall.

Depending on the level of user-interaction needed, we use two representations to train:
1. \textbf{No Interaction} We flatten the our boxes\footnote{See Supplementary for more details of the flattening process.} into a list of 5-tuples. During generation, all boxes are fully placed requiring no input from the user.
2. \textbf{User Interaction} We represent the floorplan with two sets. The first is the list of a three-tuple of box properties $\tbox$, now only containing three attributes, $\tbox = (\idxed{c}{i}, \idxed{w}{i}, \idxed{h}{i})$. The second represents the constraints between the boxes. As the final floorplan is generated by optimizing for $\idxed{x}{i}$ and $\idxed{y}{i}$ for each box, we can control the generation process by editing the constraints.

We also have a conditional generation model that can generate layouts conditioned on a specific input. We use the boundary of the layout as the condition in order to have qualitative comparisons with related work such as RPLAN\cite{Wu_DeepLayout_2019}.

\section{Furniture Layout Representation}
\label{app:furniture}

In furniture layouts, each element represents a piece of furniture with an oriented bounding box $E=(\tau, x, y, w, h, \alpha)$ that is parameterized by the type of furniture $\tau$, the lower-left corner of the bounding box $(x,y)$, the width and height of the bounding box $(w,h)$, and its orientation $\alpha$.
Three types of edges in $\mathbf{R}^C$ define adjacency, same size constraints, and same orientation constraints. \paul{TODO: check if this is the final set of constraints we will use}.
%An example is shown in Figure~\ref{fig:layout_examples}, right.

The element constraint model described in Section~\ref{sec:element_constraint_model} generates constraints $N^C = (\tau, x, y, w, h, \alpha)$ for all parameters of a furniture piece.

\section{Architecture Details}
\label{app:architecture}

\section{Optimization}
\label{app:optimization}

\paragraph{Floor plans}
In floor plans, the $x,y,w,h$ parameters of each element are bounded between their maximum and minimum values; we use $[0, 64]$ as bounds in our experiments.

The layout width $W$ is computed by first topologically sorting the elements in the subgraphs formed by horizontal adjacency edges, and then defining $W \coloneqq x_m + w_m$ for the last (right-most) element $E_m$ in the topological sort. $H$ is computed analogously. Note that we do not define $W \coloneqq \max_i x_i + w_i$ to avoid the additional constraints needed to optimize over the maximum of a set.

Each element constraint $E^C$ adds constraints of the form $v^C (1-\epsilon) \leq v \leq v^C (1+\epsilon)$, for each value $v^C$ in the element constraint $E^C$ and corresponding value $v$ in the element $E$. In our experiments, we set $\epsilon = 0.1$.

Horizontal adjacency edges $R = (E_i, E_j, \rho)$ add constraints of the form $x_i + w_i = x_j$, and analogously for vertical adjacency edges.

\paragraph{Furniture layouts}
In furniture layouts, \paul{TODO: describe optimization in furniture layouts}

\section{Training Setup}
\label{app:training_setup}
All models are trained with a cross-entropy loss with teacher forcing, i.e. providing ground truth for the previous elements in the sequence as input. The label for the $n$-th element of the input sequence is the $(n+1)$-th element of the same sequence. All input sequences are padded with special $start$ and $stop$ tokens to indicate the beginning and end of a sequence respectively. With this setting, we seek to maximize the (log-) probability of our observed sequences. The probability distribution in this case being described over $L+2$ elements, for the $L$-levels and the two special tokens.
